# Supplementary material for: Visualizing Random Forest with Self-Organising Map
Source: arXiv:1405.6684 source file (2014-05-26)
Supplement: Supplementary file 1 [file som_pima_2.pdf]

X

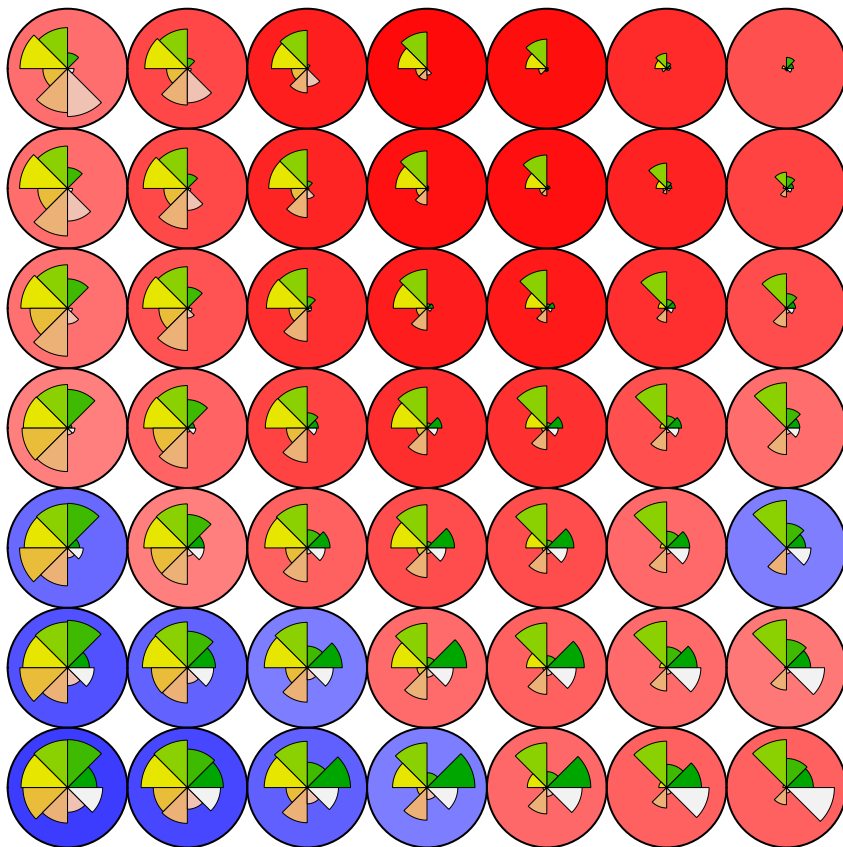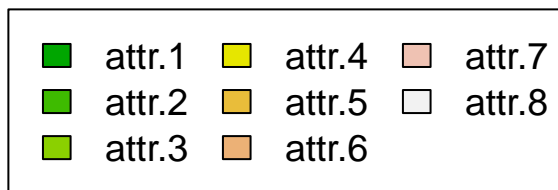

Y

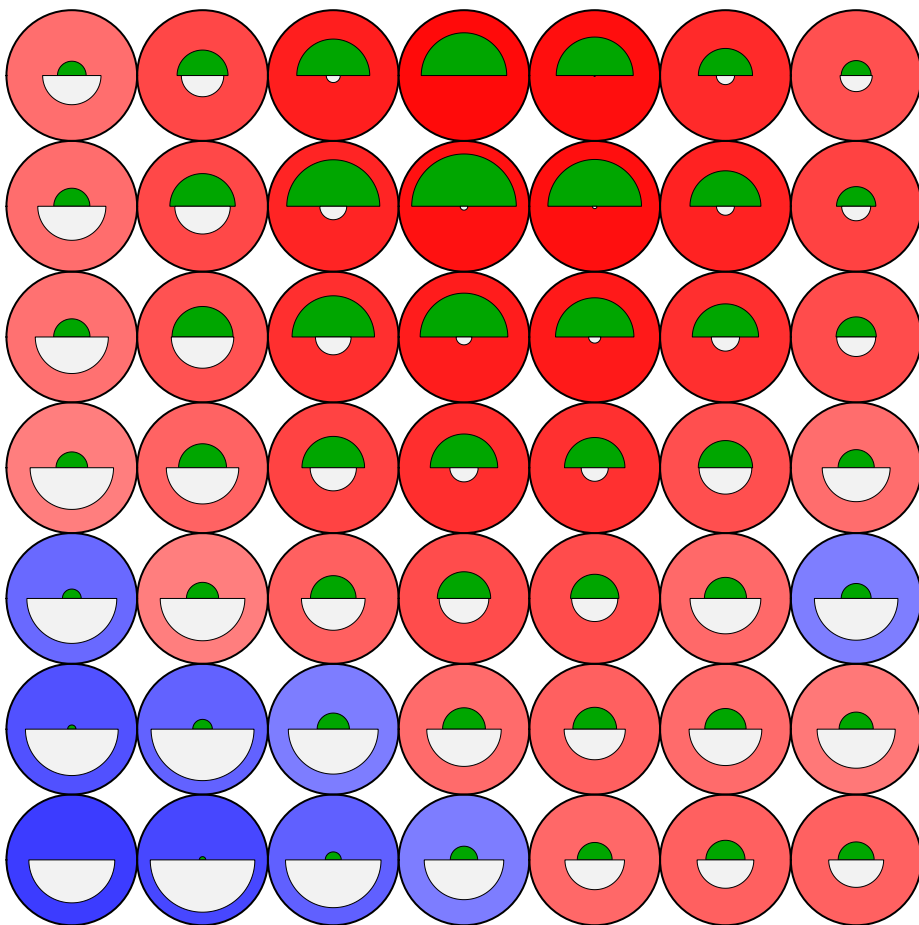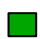

class.1

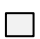

class.2
